# Supplementary material for: Stochastic Bandits with Linear Constraints
Source: arXiv:2006.10185 source file (2020-06-17)
Supplement: Supplementary file 1 [file appendix_lp_structure.tex]

\section{Supporting Lemmas}

\begin{lemma}\label{lemma::approximation_inverse_prob}
Let $x \in [0,1/2]$, and $\delta \in [-1/4, 1/4]$. Then: 

\begin{equation*}
    \left| \frac{1/2}{1/2+x+\delta} - \frac{1/2}{1/2+x}\right| \leq 4\delta
\end{equation*}
\end{lemma}

\begin{proof}
Let's start by considering the case when $\delta > 0$. Let $f_x(x) =  \frac{1/2}{1/2+x} -  \frac{1/2}{1/2+x+\delta} $. Notice that $f_x(x) \geq 0$ for all $x$. This function's derivative satisfies:
\begin{equation*}
    \frac{\partial f_x(x)}{\partial x} =  \frac{1/2}{(1/2+x+\delta)^2}  - \frac{1/2}{(1/2+x)^2}
\end{equation*}

Therefore, and since $\frac{\partial f_x(x)}{\partial x} < 0$ the function $f_x$ is decreasing and therefore the maximizer of $f_x(x)$ for $x \in [0, \frac{1}{2}]$ happens at $x = 0$. In this case:
\begin{align*}
    f_x(0) &= 1 - \frac{1/2}{1/2 + \delta} \\
    &= 1 - \frac{1}{1 + 2\delta} \\
    &= \frac{2\delta }{1+2\delta} \\
    &\leq 2\delta
\end{align*}

Now let's consider the case when $\delta < 0$. Let $f_x(x) = \frac{1/2}{1/2+x+\delta} - \frac{1/2}{1/2 + x}$. Notice that $f_x(x) \geq 0$ for all $x$. This function's derivative satisfies:
\begin{equation*}
    \frac{ \partial f_x(x)}{\partial x} = \frac{1/2}{(1/2+x)^2} - \frac{1/2}{(1/2+x+\delta)^2} 
\end{equation*}
Therefore, and since $\frac{ \partial f_x(x)}{\partial x} < 0$ the function $f_x$ is decreasing and therefore the maximizer of $f_x(x)$ for $x \in [0,\frac{1}{2}]$ happens at $x= 0$. In this case:
\begin{align*}
    f_x(0) &= \frac{1/2}{1/2 + \delta} - 1 \\
    &= \frac{-\delta}{1/2 + \delta} \\
    &\leq -4\delta
\end{align*}
The inequality follows because $1/2+ \delta \geq \frac{1}{4}$. The result follows.
\end{proof}

\section{LP structure}

Recall the optimal policy linear program \ref{eq::no_noise_LP}:
\begin{align*}\label{eq::no_noise_LP_appendix}\tag{P}
    &\mathrm{maximize} \sum_{a \in \mathcal{A}} \pi_a \bar{r}_a  \\
    \text{s.t. } & \sum_{a \in \mathcal{A}} \pi_a \bar{o}_a \geq \tau, \quad \pi \in \mathrm{\Delta}_K\\
\end{align*}
Let $\lambda_1$ and $\lambda_2$ be the two Lagrange associated with the feasibility and the simplex constraints respectively. The lagrangian of \ref{eq::no_noise_LP} takes the form:
\begin{equation*}
    L(\pi, \lambda_1, \lambda_2) = \sum_{a} \pi_a \bar{r}_a + \lambda_1\left(\sum_a \pi_a \bar{o}_a     \right) + \lambda_2\left( \sum_a \pi_a - 1 \right)
\end{equation*} 
Where $\lambda \geq 1$ and $\lambda_2 \in \mathbb{R}$. The dual function equals:
\begin{align*}
    g(\lambda_1, \lambda_2) &= \max_{\pi \geq 0} \sum_a \pi_a \bar{r}_a + \lambda_1\left(\sum_a \pi_a \bar{o}_a - \tau   \right)  + \lambda_2 \left(\sum_a \pi_a - 1 \right)  \\
    &= \max_{\pi \geq 0} \left(  \sum_a \pi_a \left( \bar{r}_a + \lambda_1 \bar{o}_a + \lambda_2 \right)   \right)-\tau \lambda_1 -\lambda_2
\end{align*}

If for any $a \in \mathcal{A}$ the expression $\bar{r}_a + \lambda_1 \bar{o}_a + \lambda_2 > 0$, then the expression inside the max will go to infinity. Therefore the dual problem equals:
\begin{align*}\label{eq::no_noise_dual_appendix}\tag{Dual}
&\min -\tau \lambda_1 - \lambda_2 \\
\text{s.t. }& \bar{r}_a + \lambda_1 \bar{o}_a + \lambda_2 \leq 0 \quad \forall a\in\mathcal{A}\\
&\lambda_1 \geq 0, \quad \lambda_2 \in\mathbb{R}
\end{align*}

Alternatively this program can be written as:

\begin{align*}
    &-\max \tau\lambda_1 + \lambda_2 \\
    \text{s.t.} & \bar{r}_a + \lambda_1 \bar{o}_a + \lambda_2 \leq 0 \quad \forall a \in \mathcal{A}
\end{align*}
Let $(\lambda_1^*, \lambda_2^*)$ be the optimal solutions for this linear program. An easy inspection of the formula above yields the following relationship between $\lambda_1^*$ and $\lambda_2^*$:
\begin{equation*}
\lambda_2^*= \min_a -\bar{r}_a - \bar{o}_a \lambda_1^* = -\max_a (\bar{r}_a + \bar{o}_a \lambda_1^*)
\end{equation*}
This allows us to write the objective function in terms of $\lambda_1$ only. We drop the subscript $1$ for clarity. The objective becomes:
\begin{align*}
    -\max_{\lambda \geq 0} \tau \lambda - \max_a (\bar{r}_a + \bar{o}_a \lambda)  &= -\max_{\lambda \geq 0} \min_a \left(    \lambda(\tau - \bar{o}_a  ) - \bar{r}_a   \right) \\
    &= \min_{\lambda \geq 0} \max_a \left( \lambda(\bar{o}_a - \tau) + \bar{r}_a     \right)
\end{align*}

It is easy to see from this equation that the existence of $a^*$ such that $\bar{o}_a \geq \tau$ is a requirement for primal feasibility. This formulation is easily interpretable. We can see that for all $\lambda \geq 0$, the value of $\max_a \lambda(\bar{o}_a - \tau) + \bar{r}_a$ upper bounds the value of any feasible policy.

\subsection{Multiple constraints}

\begin{lemma}\label{lemma::multiple_constraints_support}
The support of a multiple constraint problem equals ... 
\end{lemma}

\section{Stability of the optimal solutions}

In this section we explore the stability properties of the optimal solutions of the linear programs \ref{eq::no_noise_LP} and \ref{eq::noisy_LP}. Observe that

\subsection{Bounding the dual variable}

The following LP solves for the $l_1$ norm of $\lambda$:

\begin{align*}
    \min \lambda \\
    a 
\end{align*}
