# Supplementary material for: Stochastic Bandits with Linear Constraints
Source: arXiv:2006.10185 source file (2020-06-17)
Supplement: Supplementary file 5 [file contrained_muli_armed_bandit_appendix.tex]

\section{Constrained Multi-Armed Bandits}
\label{section::constrained_multi_armed_bandit_setup}
