# Supplementary material for: Stochastic Bandits with Linear Constraints
Source: arXiv:2006.10185 source file (2020-06-17)
Supplement: Supplementary file 6 [file optimism_pessimism_MAB_appendix.tex]

\subsection{Optimism Pessimism}\label{section::appendix_MAB_optimism_pessimism_algorithm}

Here we reproduce the full pseudo-code for OPB:

{\centering
\begin{minipage}{.9\linewidth}
    \begin{algorithm}[H]
    \textbf{Input:} Number of arms $K$, constants $\alpha_r, \alpha_c \geq 1$. \\
    \For{$t=1, \ldots , T$}{
    % \If{ $t < K+1$}{
    % pull arm $t$.}
    % \Else{
    1. Compute estimates $\{u_a^r(t) \}_{a\in\mathcal A}$, $\{u_a^c(t)  \}_{a\in\mathcal A}$.  \\
    2. Form the approximate LP (\ref{eq::noisy_LP}) using these estimates.\\
    3. Find policy $\pi_t$ by solving~\eqref{eq::noisy_LP}.\\
    4. Play arm $a \sim \pi_t$ \; \\%}
     }    
     \caption{Optimism-Pessimism}
    \label{alg::optimism_pessimism}
    \end{algorithm}
\end{minipage}
}

Similar to the case of OPLB, we define $\Pi_t = \{ \pi \in \Delta_{\mathcal{A}} : \sum_{a \in \mathcal{A}} \pi_a u_a^c(t) \leq \tau \}$. We also define $\beta_a(0) = 0$ for all $a\in \mathcal{A}$. 
%In contrast to Vanilla UCB, this approach balances the competing objectives of optimism in the reward signal and pessimism in the feasibility signal. 
